# Supplementary material for: Efficient Proximal Mapping of the 1-path-norm of Shallow Networks
Source: arXiv:2007.01003 source file (2020-07-15)
Supplement: Supplementary file 2 [file appendix_various.tex]

nothing
